# Supplementary material for: Detect Everything with Few Examples
Source: arXiv:2309.12969 source file (2024-10-02)
Supplement: Supplementary file 3 [file 9.appendix.tex]

\section{Appendix}
\renewcommand{\thefigure}{A\arabic{figure}}
\setcounter{figure}{0}
\renewcommand{\thetable}{A\arabic{table}}
\setcounter{table}{0}

\subsection{Additional Experiments}
\label{apn:exp}



\subsubsection{Over-expanded Proposal Analysis}
\label{apn:large-proposal}

\InsertBoxR{0}{
\begin{minipage}{0.49\textwidth}
    \centering
    \includegraphics[width=\textwidth]{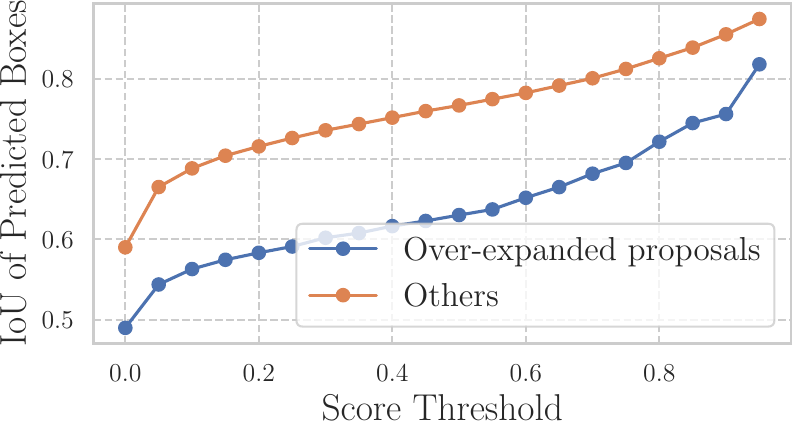}
    \vspace*{-2.5em}
    \captionof{figure}{IoU of refined bounding boxes with groundtruth objects under different score thresholds. The blue curve denotes refined boxes from over-expanded proposals.}
    \label{fig:proposal-plot}
    \vspace*{1em}
\end{minipage}}[7]

Our propagation mechanism localizes objects by first expanding the proposals and then refining the initial bounding boxes within the expanded proposals. Here we study the localization behavior of the scenario where expanded proposals cover multiple same-class objects. 
 We will use the term \emph{over-expanded proposals} to denote this scenario.

In Fig.~\ref{fig:proposal-plot}, we plot the average IoU between refined boxes and groundtruth objects under different score thresholds. A higher IoU indicates more accurate localization. It can be seen that over-expanded proposals generally degrade localization accuracy, as their final predicted boxes have smaller IoU towards the ground truth. But the degradation is far from total, e.g., they still produce boxes whose IoU $>$ 0.7 on average, under the score threshold of 0.85, which we use to generate qualitative visualizations. We also observe that the over-expanded proposals occupy around 7\% of all proposals in our model for COCO, and only half of them appear in the final prediction (after NMS and score filtering). This means even if an over-expanded proposal predicts an inaccurate box, its impact is softened by filtering of NMS and score thresholding.

In terms of actual behavior, we list success and failure cases of over-expanded proposals in Fig.~\ref{fig:proposal-multiple} and \ref{fig:proposal-multiple-bad}. In failure cases, propagation either encompasses both objects or produces erratic boxes. But all failure cases happen under inferior proposals, where the initial proposals are already poorly located and do not cover any object, or cover multiple objects before expansion. In successful cases, propagation generally prefers central objects but can locate an object accurately regardless of the proposal quality. This means our propagation localization does not fully rely on the proposal quality.


\subsubsection{Detection Accuracy at More Shots}
\label{apn:more-shots}

We study the model performance with different numbers of shots in Fig.~\ref{fig:shots} and \ref{fig:shots17}, on COCO 2014 and COCO 2017, correspondingly. For COCO 2014, the numbers of shots are set from 1 to 10, 15, 20, and 30. To align with existing work, we use the same support images by previous work~\cite{wang2020frustratingly}  for shots 2,3,5,10,30.  For other shots, we sample within the support images mentioned above. For COCO 2017, we follow the convention of the one-shot benchmark, since there does not exist a few-shot standard split of base/novel classes and preselected support images. Specifically, we compute nAP50 for all four splits and randomly select support images within the validation set of COCO 2017 for each target image. The reported nAP50 is the average among all splits and choices of support images. The numbers of shots are set from 1 to 10, 15, 20, 30, 40, 50, 75, 100.


\begin{minipage}{0.49\textwidth}
\captionof{table}{Ablation studies on annotation types used to build prototypes.}
\label{tab:ablation-bbox}
\footnotesize
\begin{tabular}{cccc}\toprule
Support Images &\multicolumn{3}{c}{nAP50} \\
Annotation &5-shot &10-shot &30-shot \\\midrule
mask &43.1 &43.1 &43.1 \\
bbox &43 &42.6 &43.1 \\
\bottomrule
\end{tabular}
\end{minipage}
\hfill
\begin{minipage}{0.49\textwidth}
    \centering
    \includegraphics[width=0.8\textwidth]{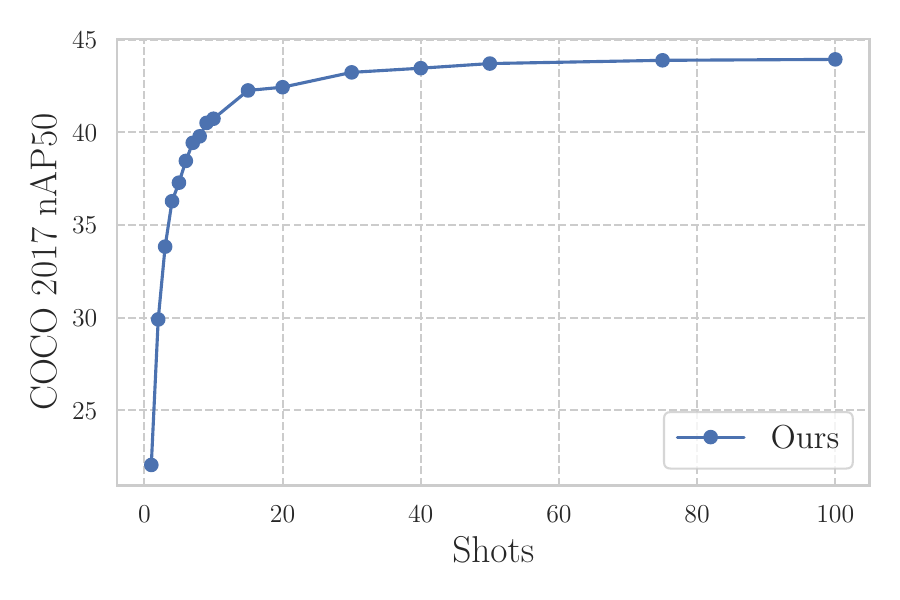}
    \vspace*{-1.5em}
    \captionof{figure}{\footnotesize Few-shot detection accuracy under different numbers of shots in COCO 2017.}
    \label{fig:shots17}
\end{minipage}



\subsubsection{Efficiency Analysis}
\label{apn:efficiency}



In Tab.~\ref{tab:effi-coco} and \ref{tab:effi-lvis}, we compare the efficiency of \mname against previous SoTA open-vocabulary methods with different values of $K$. $K$ is the number of classes ($K$) chosen to predict probability during class preselection. Our main results are obtained using $K=10$ and the result in Tab.~\ref{tab:effi-coco} is obtained using $K=3$.
The inference time of all methods is measured under the same machine with PyTorch 1.13 and a single A100 GPU. 
Similar to RegionCLIP~\cite{regionclip2022}, \mname requires a pretrained and frozen region proposal network. Recent works like F-VLM~\cite{kuo2022f} and FC-CLIP~\cite{yu2023convolutions} propose to train detectors directly on top of a frozen backbone without an additional RPN. 
However, our region proposal network involves a small computation cost. In our model for LVIS, RPN has only 27M parameters, and the number of parameters for the ViT-L backbone is 320M. The F-VLM backbone (RN50x64) has 420M parameters. In our model for COCO, RPN has only 8M parameters. 


As shown in Tab.~\ref{tab:effi-coco} and \ref{tab:effi-lvis}, \mname outperforms SoTA while being much faster at COCO and slightly slower at LVIS when $K=3$. Note that 
OWL-ViT is implemented in JAX framework \cite{frostig2018compiling}. JAX is commonly known as faster than pytorch~\cite{jaxfast}.
We select CORA instead of CORA\textsuperscript{+} and OWL-ViT rather than F-VLM for comparison because CORA\textsuperscript{+} and the RN50x64 version of F-VLM  have not been released at the moment this paper is written.
Note that we use half-precision for ViT inference as the standard practice for vision transformers and full precision for other layers.
We conduct inference time comparisons against open-vocabulary methods in addition to few-shot methods because of their superior accuracy.



\begin{table}
\scriptsize
\begin{minipage}{0.49\textwidth}
\caption{Efficiency comparison against existing state-of-the-art on COCO OVD benchmark.}\label{tab:effi-coco}
\begin{tabular}{l|c|c|cc}\toprule
Method &Backbone &top $K$ &Novel AP50 &Secs/Img \\\midrule
\multirow{3}{*}{\mname } &\multirow{3}{*}{ViT-L/14} &1 &\textbf{47.7} &\textbf{0.22} \\
& &3 &\textbf{50.0} &\textbf{0.33} \\
(Ours)& &10 &\textbf{50.0} &0.83 \\\midrule
CORA &RN50x4 &- &41.7 &0.5 \\
\bottomrule
\end{tabular}
\end{minipage}
\hfill
\begin{minipage}{0.49\textwidth}
\centering
\caption{Efficiency comparison against existing state-of-the-art on LVIS OVD benchmark.}\label{tab:effi-lvis}
\scriptsize
\begin{tabular}{l|c|c|cc}\toprule
Method &Backbone &top $K$ &box APr &Secs/Img \\\midrule
\multirow{3}{*}{\mname } &\multirow{3}{*}{ViT-L/14 } &1 &25.4 &0.35 \\
& &3 &\textbf{32.6} &0.5 \\
(Ours)& (pytorch) &10 &\textbf{33.6} &1.58 \\\midrule
OWL-ViT &ViT-L/14 (jax) &- &31.2  &\textbf{0.42} \\
\bottomrule
\end{tabular}
\end{minipage}
\end{table}



\subsubsection{Feature Visualization of DINOv2 and CLIP} 
\label{apn:feat-vis}

 The critical distinction between \mname and OVD methods is that \mname uses visual features and represents each class by the center of visual features, while OVD methods represent each class with text features, mostly from CLIP. Therefore, we sample and visualize DINOv2 and CLIP features in Fig.~\ref{fig:cluster-vis} using UMap~\cite{mcinnes2018umap}. CLIP visual features also show excellent intra-class compactness. However, there is a huge vacuum between CLIP text and visual features, and text features are almost overlapped with each other. This indicates that the distances between text and visual features may be more susceptible to noises. This further suggests that using images to represent classes could be more promising than only using texts. 


\begin{figure}
    % \vspace*{-2em}
    \centering
    \begin{minipage}{0.49\textwidth}
        \centering
        \includegraphics[width=\textwidth]{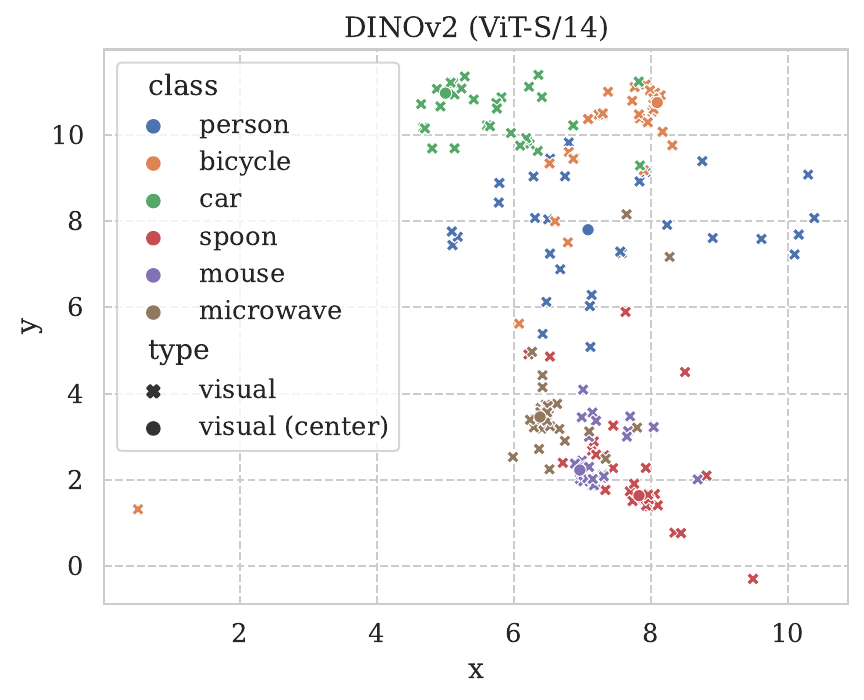}
    \end{minipage}
    \hfill
    \begin{minipage}{0.49\textwidth}
        \centering
        \includegraphics[width=\textwidth]{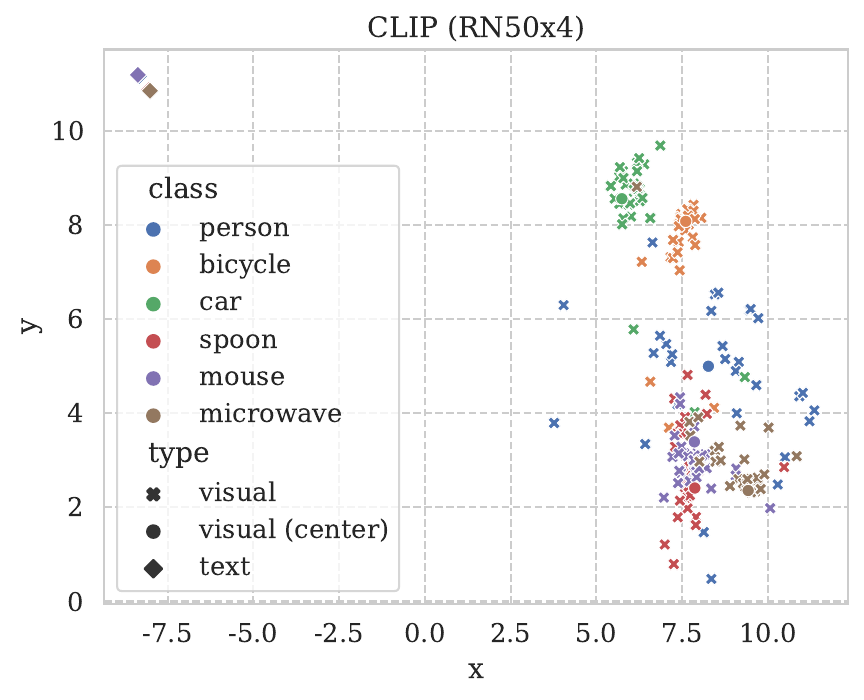}
    \end{minipage}
    \vspace*{-1em}
    \caption{Visualization of DINOv2 and CLIP (RN50x4) features in 2d plane. From visual features (\ding{54}), both DINOv2 and CLIP show good concentration within each class. However, CLIP text features (\ding{117}) locate much further from visual features. In contrast to centers of visual features (\ding{108}), text features of different classes overlap each other, showing much smaller inter-class distances. }
    %  appear to be more equally separated between classes
    \label{fig:cluster-vis}
    % \vspace*{-1em}
\end{figure}


Visual features of DINOv2 are extracted using groundtruth bounding boxes with the procedure shown in Fig.~\ref{fig:build-prototype}. 
For CLIP, we follow the standard text and region visual features extraction procedure~\cite{regionclip2022, cora2023}. Specifically, visual features are obtained by 
applying ROIAlign on the output of \texttt{res4} block. The ROIAlign outputs are fed into \texttt{res5} and attention pooling blocks to produce the final feature vector. Text features are extracted with CLIP text encoders with category names.     
We randomly sample 30 instances per class for visualization, \emph{i.e.}, each node (\ding{54}) represents an instance of the corresponding class. The UMap dimension reduction transformation is learned with a larger set of instances with both visual and text features. 



\subsection{Implementation Details}
\label{apn:more-impl-details}

\subsubsection{Network Architecture}

\begin{minipage}{0.6\linewidth}
    \centering
    \stackunder[5pt]{\includegraphics[width=0.48\textwidth]{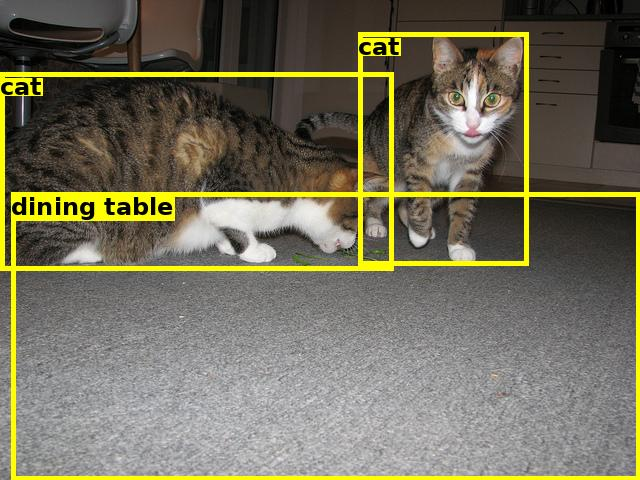}}{(a)}
    \hfill
    \stackunder[5pt]{\includegraphics[width=0.48\textwidth]{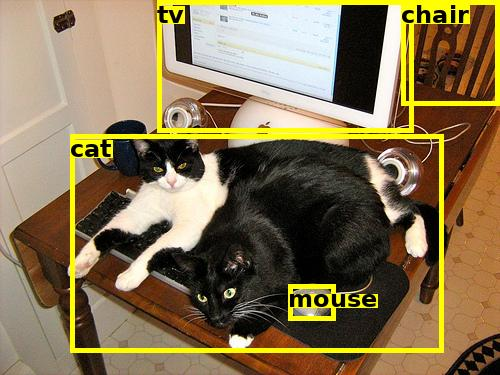}}{(b)}
    \captionof{figure}{Failure cases of our method on COCO. In the image (a), the floor is detected as a dining table, possibly due to visual similarity. In image (b), a single box covers both the two cuddling cats, likely caused by very little visual separation between the two.}
    \label{fig:bad-case}
\end{minipage}
\hfill
\begin{minipage}{0.34\linewidth}
  \includegraphics[width=\linewidth]{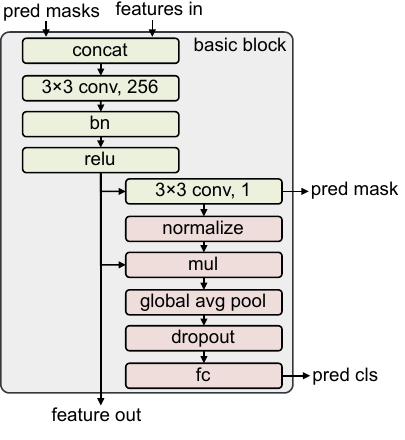}
  \vspace*{-2em}
  \captionsetup{font=footnotesize}
  \captionof{figure}{Basic building block for our RCNN networks.}
  \label{fig:net-arch}
\end{minipage}


\vspace{0.5em}

Fig.~\ref{fig:net-arch} illustrates the network building block used in our convolution neural networks for classification, localization, and instance segmentation branches. 
Sigmoid cross entropy loss and dice loss~\cite{sudre2017generalised} are applied on the mask output at each layer in the localization and segmentation branch.
The red blocks are only used in the classification branch. For the classification branch, the mask prediction serves as spatial attention and receives no supervision, similar to the squeeze-and-excitation block in SENet~\cite{hu2018squeeze} but at spatial dimensions. The input to both classification and localization branches is the similarity map between proposal features and prototypes, while the input to the instance segmentation branch for LVIS is the concatenation of similarity maps and multi-scale ViT features. 
For models trained with COCO, we use 3 blocks for classification and 5 blocks for localization. For LVIS, we use 5 blocks for all branches. 
 The \texttt{3$\times$3 conv, 256} denotes a convolution layer with kernel size 3 and 256 output channels. We use $T=128$ in the class rearrange module for both COCO and LVIS.

\subsubsection{Operations}

\noindent\textbf{Proposal Expansion.} Eq.~\ref{eq:box-expand} explains the proposal expansion block in Fig.~\ref{fig:method-localization}. $(c_w, c_h, w, h)$ and $(c^{\text{exp}}_w, c^{\text{exp}}_h, w^{\text{exp}} , h^{\text{exp}})$ represent the original the expanded proposal.

\begin{equation}
\begin{split}
& m = \min (0.4 w, 0.4 h) \\
& (w^\text{exp}, h^\text{exp}) = (w, h) + m \\
& (c_w^\text{exp}, c_h^{\text{exp}}) = (c_w, c_h)
\end{split}
\label{eq:box-expand}
\end{equation}

\noindent\textbf{Box2Heatmap.} Eq.~\ref{eq:box2heatmap} explains the Box2Heatmap block in Fig.~\ref{fig:method-localization}. $\mathbf{H} \in \mathbb{R}^{H\times W}$ represents the output heatmap. $(x_0, y_0)$ and $(x_1, y_1)$ denotes the coordinates of the left top and right bottom point of the original proposal, where $(x_0, y_0) = (c_w, c_h) - (w, h)/2$ and $(x_1, y_1) = (c_w, c_h) + (w, h)/2$ .

\begin{equation}
\mathbf{H}_{ji} = \begin{cases}
1 & (x_0^\text{exp} + \frac{i}{W} w^\text{exp}, y_0^\text{exp} + \frac{j}{H} h^\text{exp}) \in [x_0, x_1] \times [y_0, y_1] \\
0 & \text{otherwise}
\end{cases} 
\label{eq:box2heatmap}
\end{equation}

\noindent\textbf{Clustering.} The clustering algorithm used in building prototypes is initially proposed by SwAV~\cite{caron2020unsupervised} and based on optimal transport~\cite{villani2009optimal}. The optimal transport problem is an optimization problem that aims to find an optimal mapping $\gamma^* \in \mathbb{R}_+^{n\times m}$  from a source distribution $\mathbf{a} = [a_1, ..., a_n], \sum_{i=1}^n a_i = 1$ to target distribution $\mathbf{b} = [b_1, ..., b_n], \sum_{i=1}^m b_i = 1$, which minimizes the overall transport cost. Let $\mathbf{M}\in \mathbb{R}^{n\times m}$ denote the cost matrix, where $\mathbf{M}_{ij}$ denote the cost of moving mass from $a_i$ to $b_j$. This problem is formulated in Eq.~\ref{eq:ot}.


\begin{equation}
\begin{split}
& \gamma^*=\arg \min _{\gamma \in \mathbb{R}_{+}^{n \times m}} \sum_{i, j} \gamma_{ij} \mathbf{M}_{ij} \\
& \text { s.t. } \gamma \mathbf{1}= \mathbf{a} ; \gamma^T \mathbf{1}= \mathbf{b} ; \gamma \geq 0
\end{split}
\label{eq:ot}
\end{equation}

The clustering procedure consists of the iterations of two steps. First, an optimal transport $\gamma^*$ is computed between a set of centroids $\mathbf{C} \in \mathbb{R}^{c\times d}$ and instance-level prototypes $\mathbf{Q} \in \mathbb{R}^{q\times d}$, where $c$ represents the number of centroids and $q$ represents the number of instance-level prototypes for a given class in a mini-batch. Note that we apply data augmentation to generate more instance-level prototypes from a limited set of support images. The negative dot similarity $\mathbf{M} = -\mathbf{C} \mathbf{Q}^{\top}$ is used as the cost matrix, and $\mathbf{a}, \mathbf{b}$ are set as uniform. The solution $\gamma^*$ is estimated from the sinkhorn knopp algorithm~\cite{cuturi2013sinkhorn}. 
Second, a momentum update is made to the centroids with $\mathbf{C} = (1 - \beta)  \mathbf{C} + \beta \gamma^* \mathbf{Q}$, where $\beta$ is the momentum parameter. 
Clustering is applied on instance prototypes per class. We use $c=10$ and $\beta = 0.002$ for all experiments and compute the average of the 10 centroids as the prototype for each class. For background prototypes, we directly use centroids without averaging. This optimal-transport-based online clustering procedure is commonly used in prototype learning~\cite{zhou2022rethinking, wang2022visual}. In hindsight, we also try directly setting class-level prototypes as the mean of instance prototypes for each class without augmentation. This yields almost identical results on open-vocabulary experiments for both COCO and LVIS with ViT-L/14, other settings are not tested. This suggests that the details of the clustering procedure may not be a critical element within our method. 






\subsection{Visualization Details}
\label{apn:vis}


% 3-4
\noindent\textbf{Demonstration on YCB Objects.} Fig.~\ref{fig:demo} shows the detection results of \mname on YCB objects, a standard set of objects widely used in robotic manipulation benchmark~\cite{calli2015ycb}. There are misclassifications and inaccurate boxes, \emph{e.g.}, the white skillet is mistaken as a can, all round-shape fruits are recognized as orange, while the red one is clearly an apple. However, we believe the overall result is encouraging. The specification of YCB objects at the time this paper is written includes 72 categories. We use a total of 33 by selecting and merging certain categories. The categories in use are 
{\footnotesize \texttt{apple, ball, banana, bowl, brick, can, cheez-it, chips, clamp, cleanser bottle, coffee jar, comet pine, cups, drill, glass, lego, lemon, marker, mug, mustard, orange, peach, pear, peg-hole, pitcher, plate, screwdriver, skillet, spray bottle, sugar box, toy airplane box, utensil, wood blocks jar}}. The source image in Fig.~\ref{fig:demo} is taken from the banner picture of \href{https://www.ycbbenchmarks.com/}{ycbbenchmarks.com}. 
For each category, we use google image search to collect a few sample images. Fewer than four images on average are gathered per category. We annotate the corresponding objects by instance masks in each image using the software provided by SimpleClick~\cite{liu2022simpleclick}. Similar to SAM,  SimpleClick generates instance masks automatically from user clicks, which significantly simplifies and accelerates the annotation procedure. Our annotator feedback indicates that annotating masks with SimpleClick is even easier and more accurate than drawing bounding boxes. An NVIDIA 3060 GPU is used for SimpleClick software. Class prototypes for YCB objects are built from the annotated example images. During \mname inference, we replace prototypes of LVIS categories with those of YCB objects in order to detect these new categories. During postprocessing, We apply class-agnostic NMS and filter small bounding boxes. The full code and data for this demonstration will be released in our repository.




% comment on the results
% how the categories are selected
% what processing we use, limitation.

\begin{figure}[h]
    \centering
    \captionsetup[subfigure]{justification=centering,labelformat=empty}
    \subfloat[Proposal]{\includegraphics[width=0.12\textwidth]{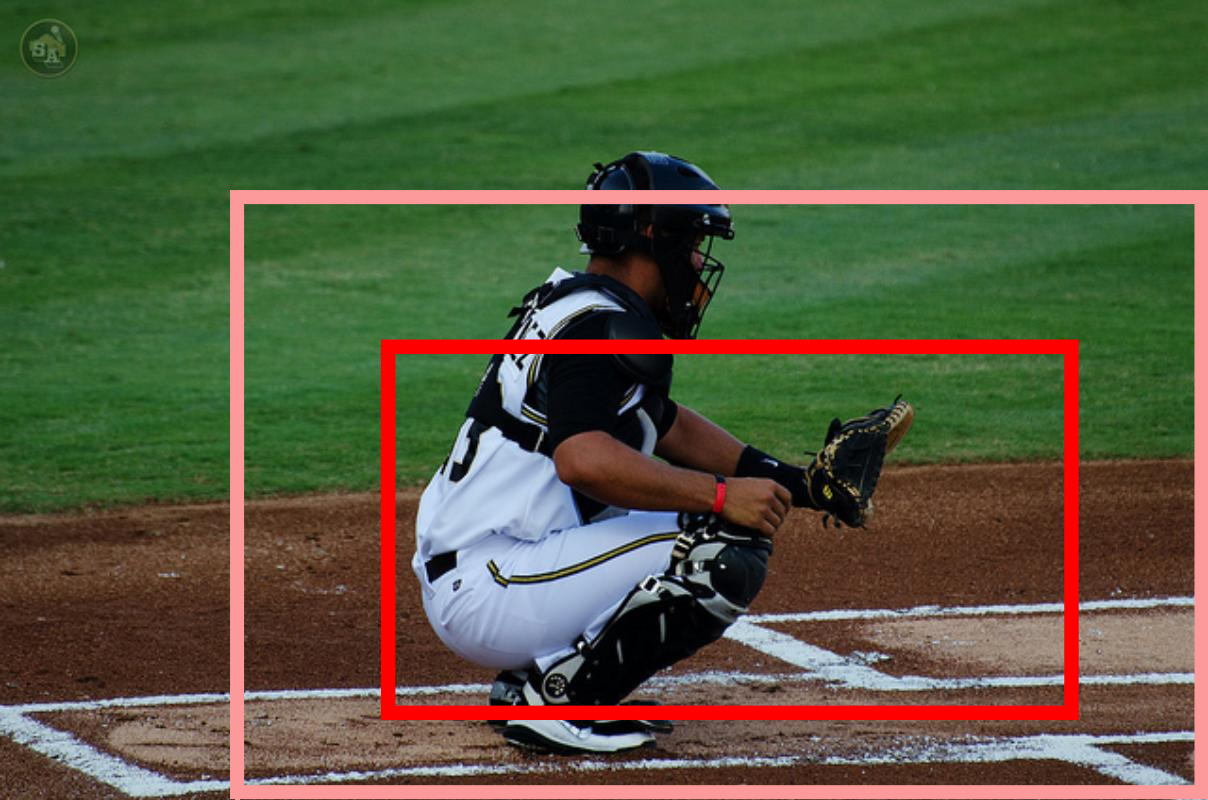}}\hfill
     \subfloat[Initial \\ Heatmap]{\includegraphics[width=0.08\textwidth]{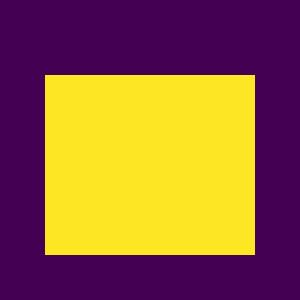}}\hfill       
      \subfloat[Propagated \\ Heatmaps]{\includegraphics[width=0.08\textwidth]{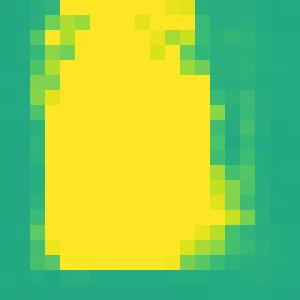}
        \includegraphics[width=0.08\textwidth]{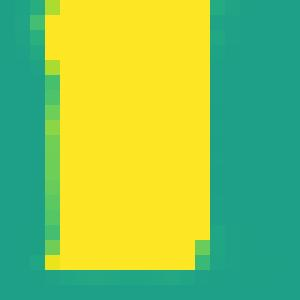} 
      }     
    \subfloat[Final \\ Prediction]{\includegraphics[width=0.12\textwidth]{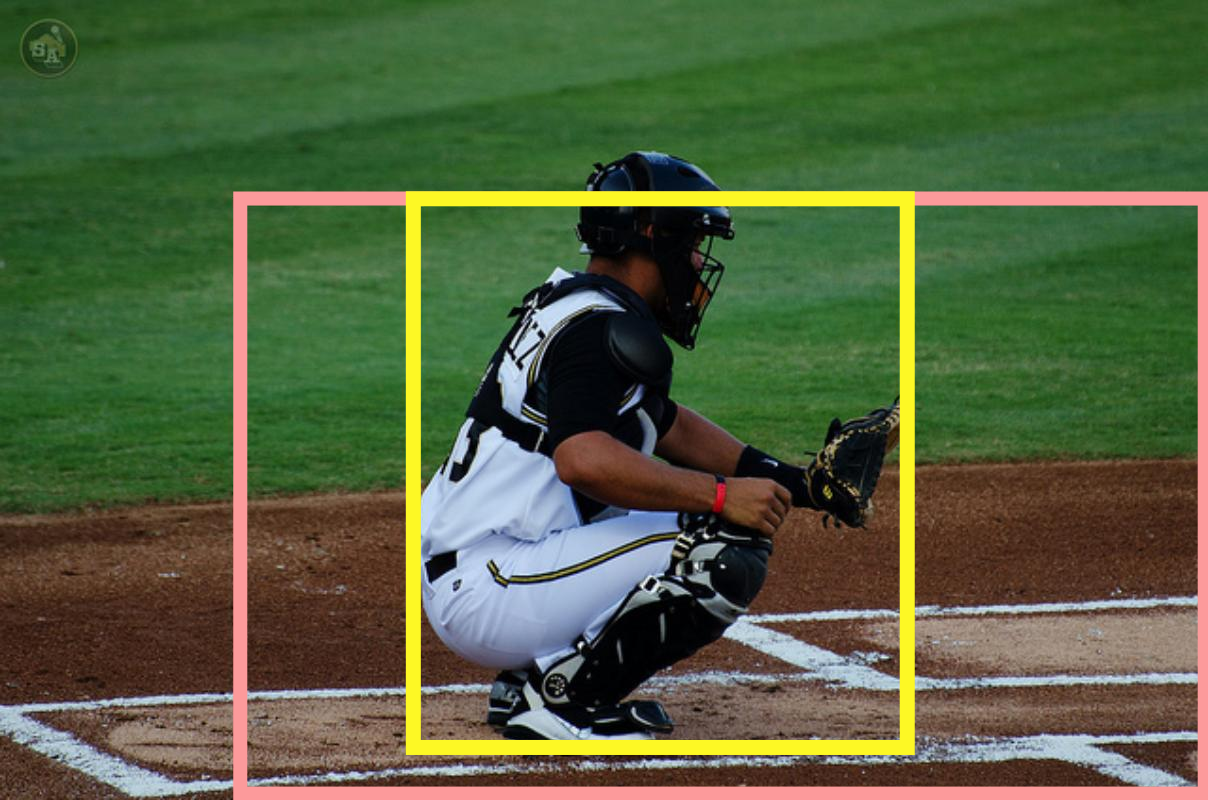}}\hfill       
    %%%%
         \subfloat[Proposal]{\includegraphics[width=0.12\textwidth]{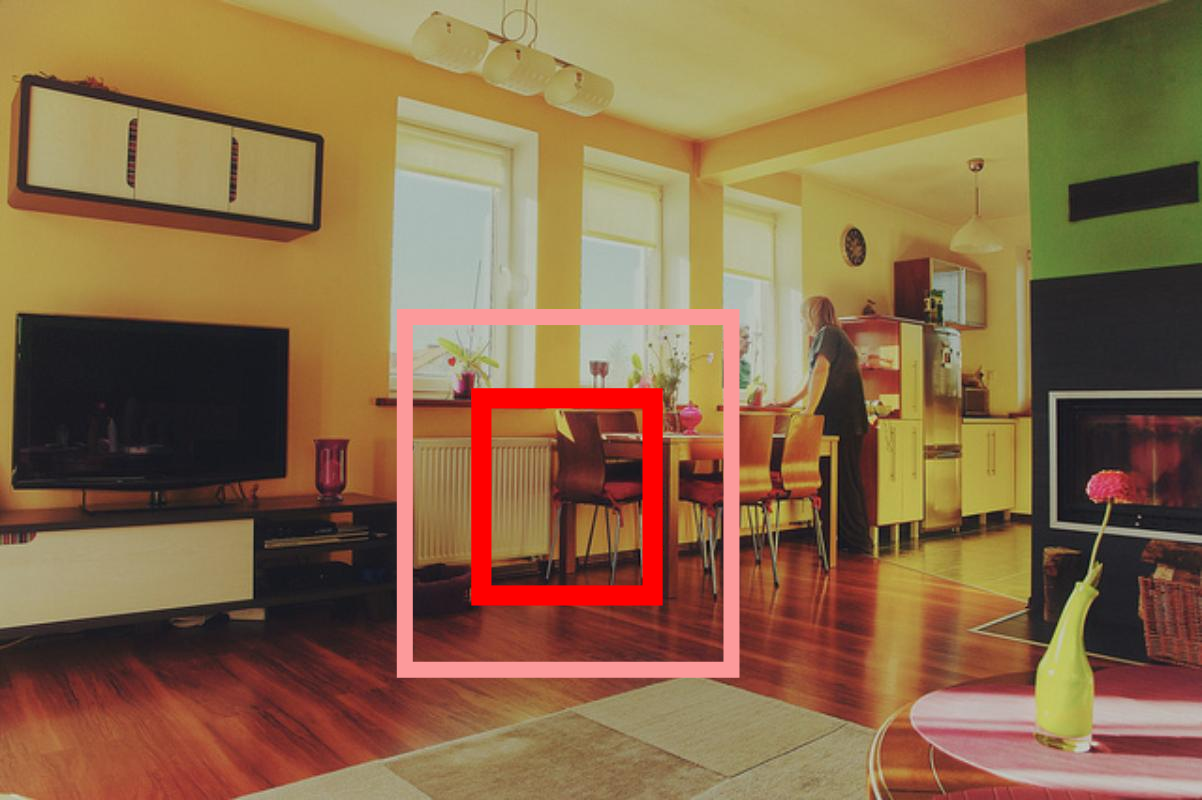}}\hfill
     \subfloat[Initial \\ Heatmap]{\includegraphics[width=0.08\textwidth]{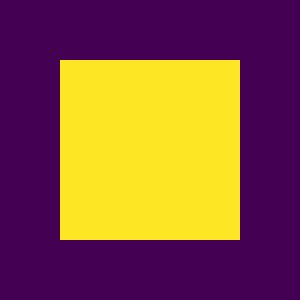}}\hfill       
      \subfloat[Propagated \\ Heatmaps]{\includegraphics[width=0.08\textwidth]{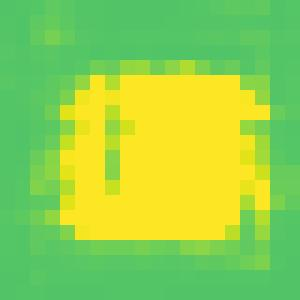} \includegraphics[width=0.08\textwidth]{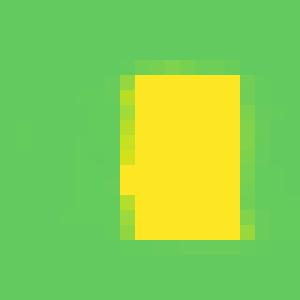}}\hfill       
    \subfloat[Final \\ Prediction]{\includegraphics[width=0.12\textwidth]{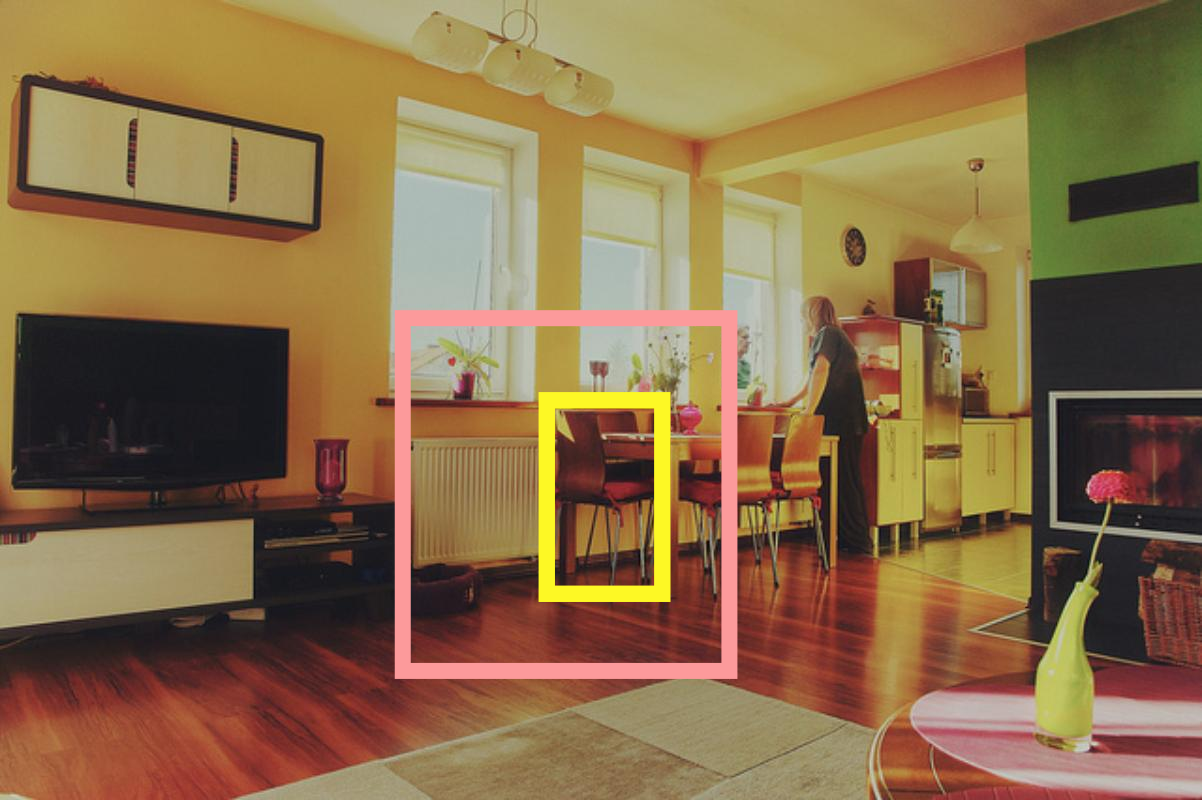}}\hfill    
    \caption{Examples of heatmaps in region propagation. The proposal, expanded proposal, and final prediction box are colored in \ulcolor[red]{red}, \ulcolor[pink]{pink}, and \ulcolor[yellow]{yellow}, respectively. The initial heatmap encodes the spatial relationship between proposals and expanded proposals in binary masks. Propagated heatmaps are softmax predictions sampled from the binary segmentation network in our region propagation architecture. }
    \label{fig:region-prop}
\end{figure}






\noindent\textbf{Region Propagation.} Fig.~\ref{fig:region-prop} visualizes the heatmap changes of sampled detection results during region propagation. A clear mapping can be found between the detection bounding boxes and the corresponding salient regions within the expanded proposal. The softmax predictions are normalized by dividing mean values in order to enhance the visual quality.





\begin{figure}
    \centering
    \includegraphics[\linewidth]{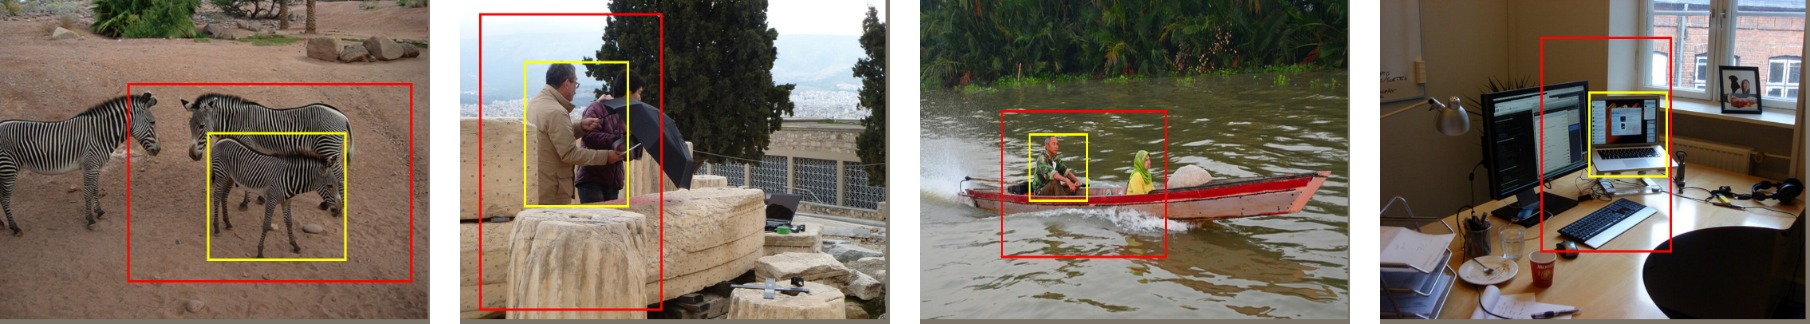}
  \vspace{-1.5em}
    \caption{Successful cases of our propagation-based localization under over-expanded proposals. The expanded proposals and final prediction boxes are colored in \ulcolor[red]{red} and \ulcolor[yellow]{yellow}, correspondingly. It can be seen that propagation generally prefers central objects, but can locate an object accurately even if the object is not located at the center of the proposal.
    }
    \label{fig:proposal-multiple}
\end{figure}

\begin{figure}
    \centering
    \includegraphics[\linewidth]{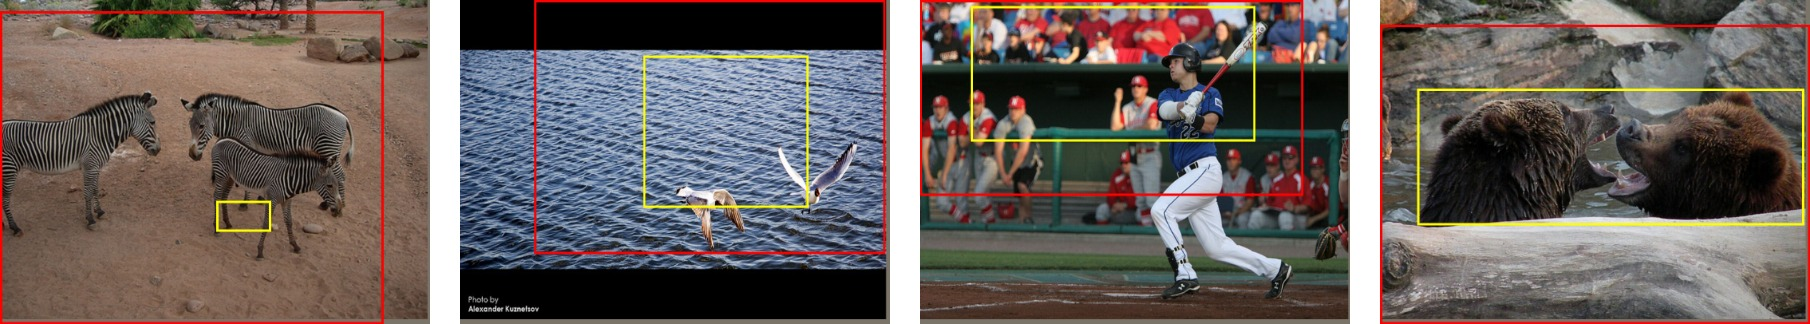}
    \vspace{-1.5em}
    \caption{Failure cases of our propagation-based localization under over-expanded proposals. The propagation either encompasses both objects, or produces erratic boxes. But all failure cases happen under inferior proposals, where the proposals are already poorly located and do not cover any object, or cover multiple objects before expansion.}
    \label{fig:proposal-multiple-bad}
\end{figure}

\begin{figure}[h]
    \centering
    \captionsetup[subfigure]{justification=centering,labelformat=empty}
    
    \subfloat[]{\includegraphics[width=0.33\textwidth]{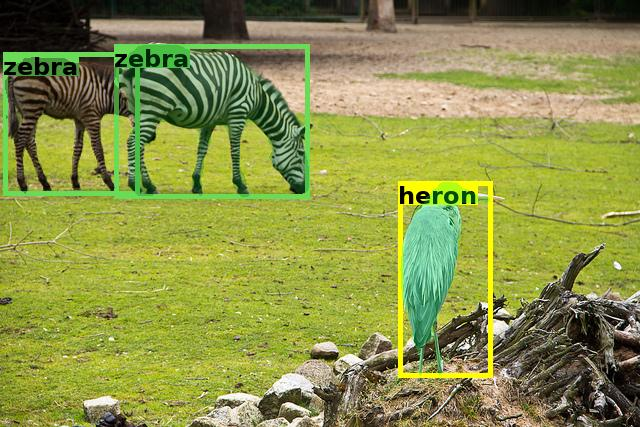}}\hfill
    \subfloat[]{\includegraphics[width=0.33\textwidth]{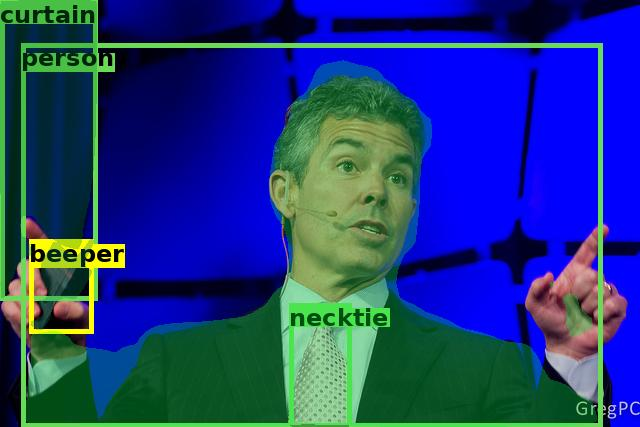}}\hfill
    \subfloat[]{\includegraphics[width=0.33\textwidth]{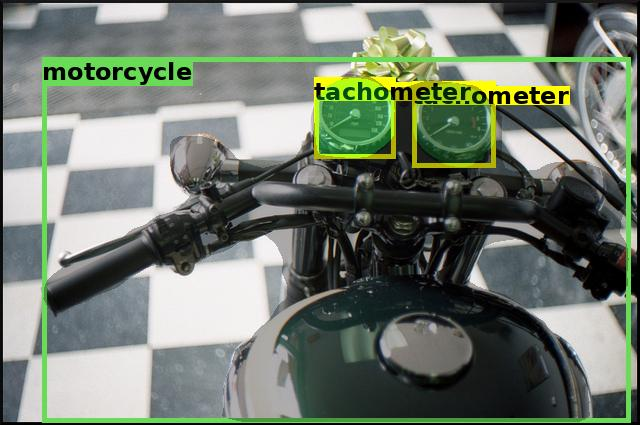}}\hfill
    \vspace{-2em}

    \subfloat[]{\includegraphics[width=0.33\textwidth]{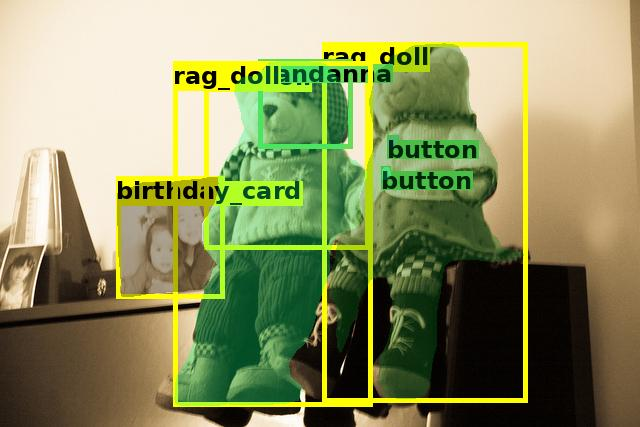}}\hfill
    \subfloat[]{\includegraphics[width=0.33\textwidth]{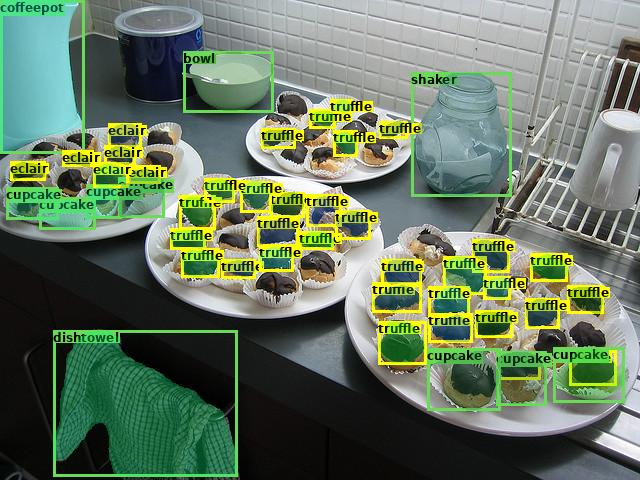}}\hfill
    \subfloat[]{\includegraphics[width=0.33\textwidth]{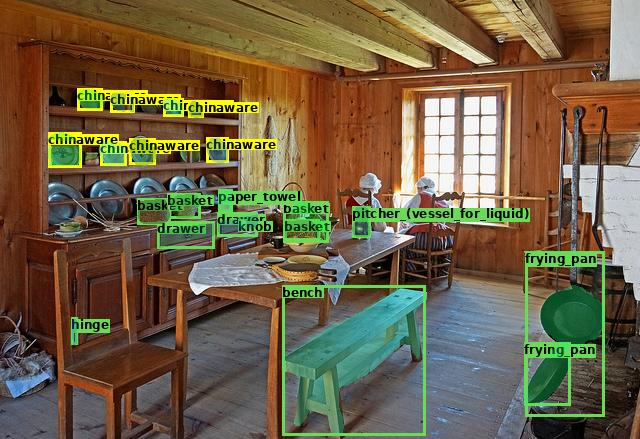}}\hfill
    
    \vspace{-1.5em}
    \caption{Qualitative visualization of our method DE-ViT on LVIS. Boxes of base and novel classes are colored in \ulcolor[green]{green} and \ulcolor[yellow]{yellow}, correspondingly.}
    \label{fig:lvis-q}
\end{figure}


\begin{figure}[h]
    \centering
    \captionsetup[subfigure]{justification=centering,labelformat=empty}

    \rotatebox{90}{\hspace{3em} Ours}
    \subfloat[]{\includegraphics[width=0.31\textwidth]{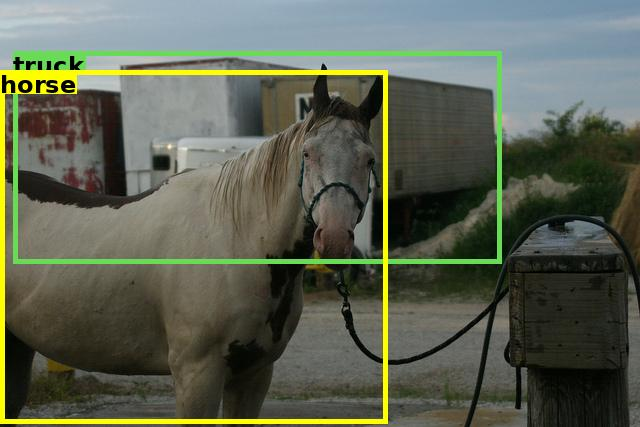}}\hfill
        \subfloat[]{\includegraphics[width=0.31\textwidth]{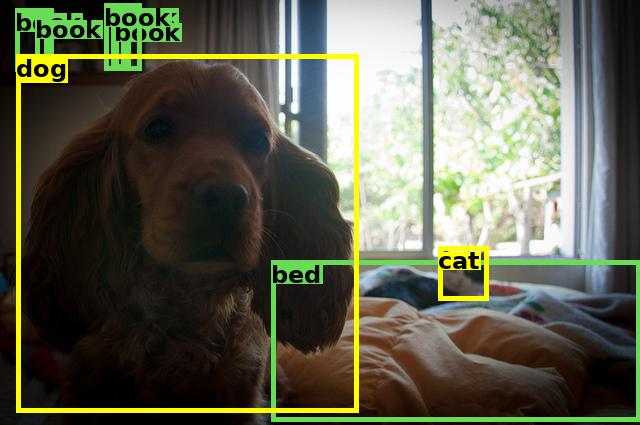}}\hfill
         \subfloat[]{\includegraphics[width=0.31\textwidth]{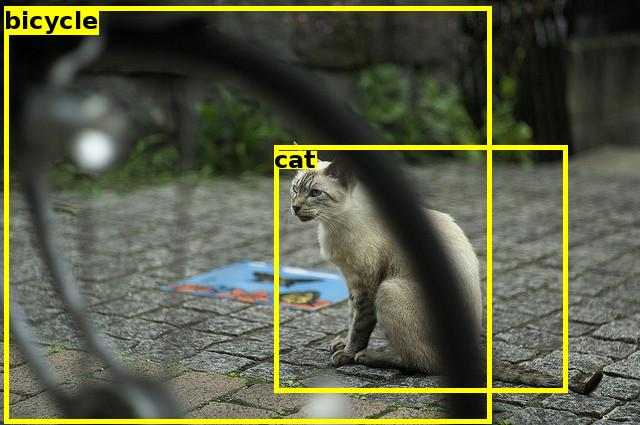}}\hfill
 
    \vspace{-2em}
    
     \rotatebox{90}{\hspace{0.2em} Meta Faster RCNN}
     \subfloat[]{\includegraphics[width=0.31\textwidth]{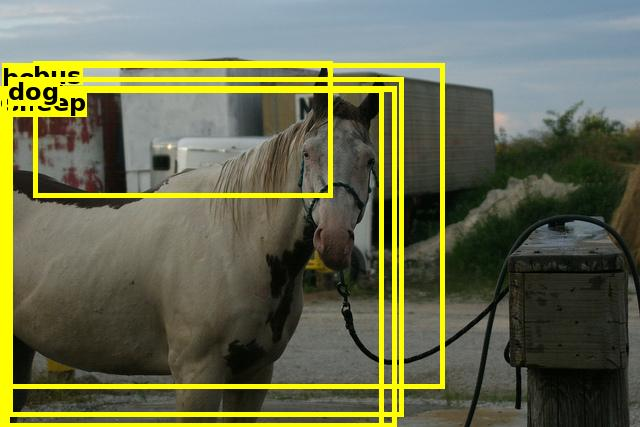}}\hfill
       \subfloat[]{\includegraphics[width=0.31\textwidth]{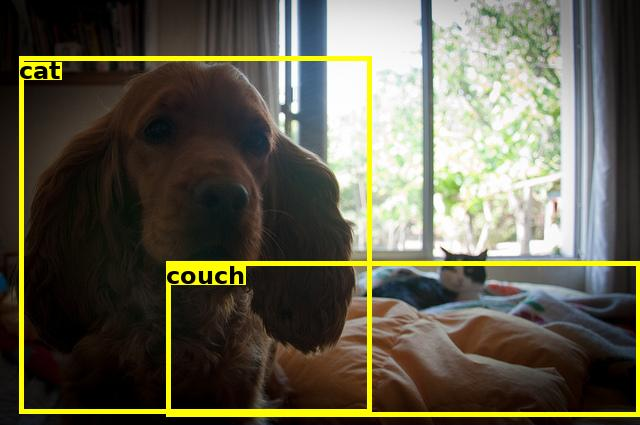}}\hfill
        \subfloat[]{\includegraphics[width=0.31\textwidth]{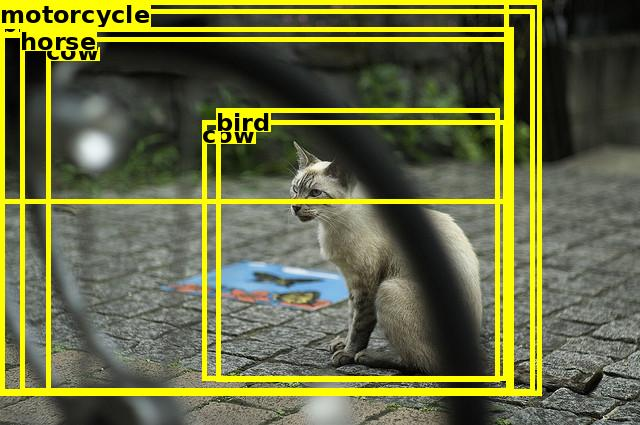}}\hfill
     \vspace{-1.5em}
    \caption{Qualitative comparison between our method DE-ViT with few-shot detector Meta Faster RCNN~\cite{han2022meta} in COCO.
     DE-ViT detects more novel objects while having much fewer false positives. Note that Meta Faster RCNN can only detect novel objects after finetuning over novel classes, while our method can detect both base and novel classes without any finetuning. Boxes of base and novel classes are colored in \ulcolor[green]{green} and \ulcolor[yellow]{yellow}, correspondingly.}
    \label{fig:coco-14-more-q}
\end{figure}


\begin{figure}[h]
    \centering
    \captionsetup[subfigure]{justification=centering,labelformat=empty}

    \rotatebox{90}{\hspace{3em} Ours}
    \subfloat[]{\includegraphics[width=0.31\textwidth]{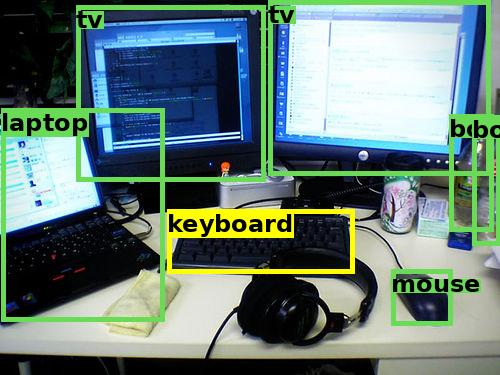}}\hfill
        \subfloat[]{\includegraphics[width=0.31\textwidth]{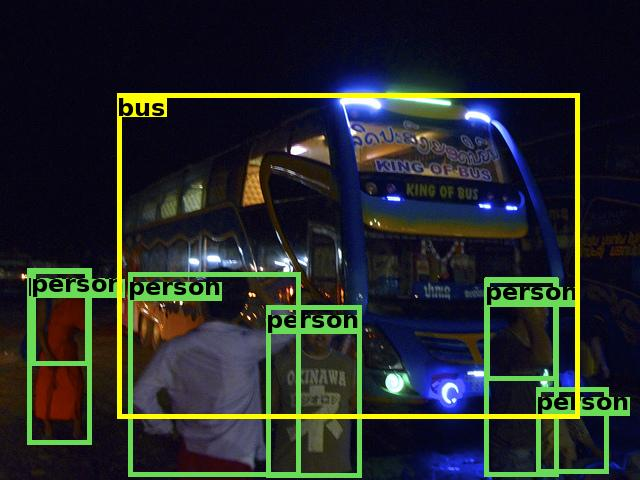}}\hfill
         \subfloat[]{\includegraphics[width=0.31\textwidth]{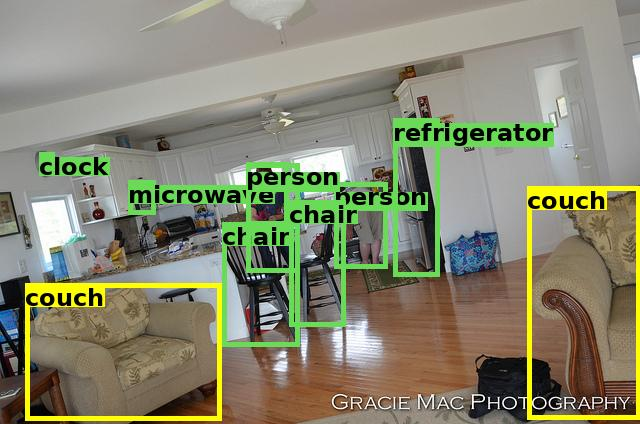}}\hfill
 
    \vspace{-2em}
    
     \rotatebox{90}{\hspace{2.8em} CORA}
     \subfloat[]{\includegraphics[width=0.31\textwidth]{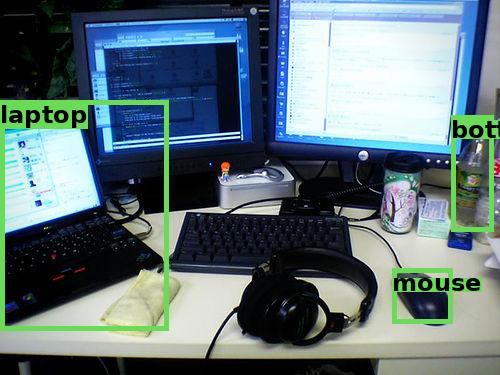}}\hfill
       \subfloat[]{\includegraphics[width=0.31\textwidth]{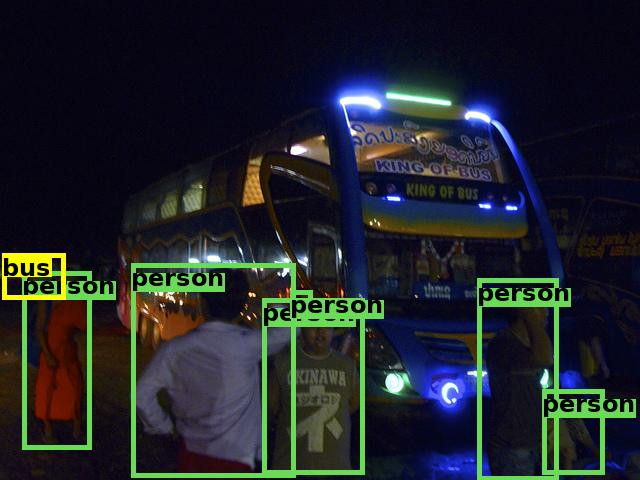}}\hfill
        \subfloat[]{\includegraphics[width=0.31\textwidth]{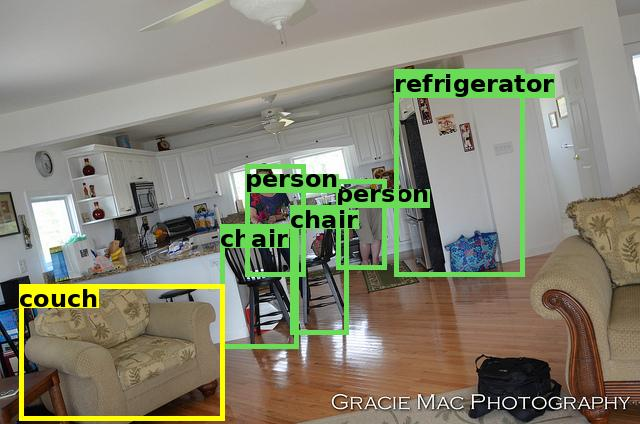}}\hfill

    \caption{Qualitative comparison between our method DE-ViT with open-vocabulary detector CORA~\cite{cora2023} in COCO. Boxes of base and novel classes are colored in \ulcolor[green]{green} and \ulcolor[yellow]{yellow}, correspondingly.}
    \label{fig:coco-17-more-q}
\end{figure}
